# Supplementary material for: Seniority and Hierarchy Configuration Interaction for Radicals and Excited States
Source: arXiv:2308.14618 ancillary file (2023-11-15)
Supplement: Supplementary file 1 [file sup.pdf]

# Supporting Information for “Seniority and Hierarchy Configuration Interaction for Radicals and Excited States”

Fábris Kossoski[1, a)] and Pierre-François Loos[1, b)]

*Laboratoire de Chimie et Physique Quantiques (UMR 5626), Université de Toulouse, CNRS, UPS, France*

[a)]Electronic mail: fkossoski@irsamc.ups-tlse.fr

[b)]Electronic mail: loos@irsamc.ups-tlse.fr

Given two sets of $N$ paired variables $x_i$ and $y_i$ (in our case, the approximate and reference excitation energies), the corresponding mean signed error (MSE), mean absolute error (MAE), root-mean-square error (RMSE), and standard deviation of the errors (SDE) are defined as:

$$\text{MSE} = \frac{1}{N}\sum_{i=1}^{N}(x_i - y_i), \tag{S1a}$$

$$\text{MAE} = \frac{1}{N}\sum_{i=1}^{N}|x_i - y_i|, \tag{S1b}$$

$$\text{RMSE} = \sqrt{\frac{1}{N}\sum_{i=1}^{N}(x_i - y_i)^2}, \tag{S1c}$$

$$\text{SDE} = \sqrt{\frac{1}{N}\sum_{i=1}^{N}(x_i - \mu)^2}, \tag{S1d}$$

where

$$\mu = \frac{1}{N}\sum_{i=1}^{N} x_i. \tag{S2}$$

Equilibrium geometry of ethylene, in atomic units, obtained from Ref. 1:

```
C    0.00000000       1.26026583       0.00000000
C    0.00000000      -1.26026583       0.00000000
H    0.00000000       2.32345976       1.74287672
H    0.00000000      -2.32345976       1.74287672
H    0.00000000       2.32345976      -1.74287672
H    0.00000000      -2.32345976      -1.74287672
```

Equilibrium geometry of vinyl, in atomic units, obtained from Ref. 2:

```
C    0.00000000       1.16769663      -0.04303146
C    0.00000000      -1.29945364       0.15810072
H    0.00000000       2.38429609       1.59801822
H    0.00000000       2.08759130      -1.87998309
H    0.00000000      -2.90307925      -1.08814513
```

By fitting the computed potential energy curves with a Morse potential $V(r) = D[1-e^{-a(r-r_e)}]^2+C$, we obtained equilibrium geometries $r_e$, force constants $2Da^2$, and harmonic vibrational frequencies $\left(Da^2/2\pi^2\mu\right)^{1/2}$, where $\mu$ is the reduced mass. Since the fitting is restricted to the equilibrium region, employing more elaborate functions would be inconsequential, such that the adopted Morse potential is well justified. The fitting was performed with the Marquardt-Levenberg algorithm implemented in GNUPLOT. The following intervals have been considered for the fitting:

- HF: 0.8 Å to 1.3 Å
- $F_2$: 1.25 Å to 1.65 Å
- ethylene: 2.2 $a_0$ to 2.9 $a_0$
- $N_2$: 0.95 Å to 1.3 Å
- $H_4$: 1.45 $a_0$ to 1.95 $a_0$
- $H_8$: 1.6 $a_0$ to 2.05 $a_0$
- OH: 0.85 Å to 1.2 Å
- CN: 1.0 Å to 1.4 Å
- vinyl: 2.35 $a_0$ to 2.7 $a_0$
- $H_7$: 1.6 $a_0$ to 2.05 $a_0$

The non-parallelity error and distance error were computed for the following intervals:

- HF: 0.5 Å to 6 Å
- $F_2$: 0.95 Å to 8 Å
- ethylene: 1.5 $a_0$ to 16 $a_0$
- $N_2$: 0.7 Å to 4 Å
- $H_4$: 1 $a_0$ to 10 $a_0$
- $H_8$: 1 $a_0$ to 10 $a_0$
- OH: 0.6 Å to 8 Å
- CN: 0.7 Å to 4 Å
- vinyl: 1.7 $a_0$ to 9 $a_0$
- $H_7$: 1 $a_0$ to 10 $a_0$

TABLE S1. Number of Determinants in Hierarchy-, Excitation, and Seniority-Based CI Routes, as well as in Full CI, for OH, CN, vinyl, and $H_7$, with the cc-pVDZ basis set and frozen-core approximation.

| method | OH | CN | vinyl | $H_7$ |
|---|---|---|---|---|
| RHF | 1 | 1 | 1 | 1 |
| CIS | 131 | 280 | 533 | 221 |
| CISD | 5 871 | 27 559 | 100 983 | 16 403 |
| CISDT | 110 031 | 1 196 384 | 8 620 123 | 491 695 |
| CISDTQ | 1 035 501 | 27 468 434 | 397 093 838 | 7 015 800 |
| CIs1 | 58 140 | 8 288 280 | 1 160 068 104 | 209 440 |
| CIs3 | 1 686 060 | 530 449 920 | 143 268 410 844 | 9 948 400 |
| CIs5 | 12 267 540 | 9 233 143 920 | 4 974 952 064 004 | 107 338 000 |
| hCI1 | 299 | 658 | 1 268 | 500 |
| hCI1.5 | 3 491 | 11 809 | 35 813 | 11 009 |
| hCI2 | 25 401 | 136 234 | 569 178 | 96 290 |
| hCI2.5 | 162 265 | 1 417 234 | 8 899 178 | 832 850 |
| hCI3 | 732 107 | 10 879 834 | 102 007 753 | 5 530 745 |
| hCI3.5 | 2 706 807 | 71 632 834 | 1 011 139 788 | 23 829 890 |
| hCI4 | 7 774 870 | 384 458 809 | 8 484 940 738 | 92 360 660 |
| FCI | 45 070 128 | 446 075 229 600 | 4 672 770 853 882 482 | 342 696 200 |

TABLE S2. Number of Determinants in Hierarchy-, Excitation, and Seniority-Based CI Routes, as well as in Full CI, for $H_4$, $N_2$, and $F_2$, with the cc-pVDZ basis set and frozen-core approximation.

| method | $H_4$ | $N_2$ | $F_2$ |
|---|---|---|---|
| RHF | 1 | 1 | 1 |
| CIS | 73 | 211 | 267 |
| CISD | 1 675 | 15 436 | 25 138 |
| CISDT | 12 691 | 483 036 | 1 048 174 |
| CISDTQ | 36 100 | 7 745 886 | 23 236 165 |
| CIs0 | 190 | 65 780 | 657 800 |
| CIs2 | 7 030 | 6 972 680 | 88 145 200 |
| CIs4 | 36 100 | 145 110 680 | 2 450 305 000 |
| hCI1 | 109 | 316 | 400 |
| hCI1.5 | 757 | 2 836 | 3 592 |
| hCI2 | 3 052 | 34 336 | 57 457 |
| hCI2.5 | 17 740 | 311 536 | 531 469 |
| hCI3 | 36 100 | 1 913 836 | 4 209 850 |
| hCI3.5 | 36 100 | 11 489 836 | 28 628 650 |
| hCI4 | 36 100 | 49 045 711 | 153 775 000 |
| FCI | 36 100 | 4 327 008 400 | 432 700 840 000 |

TABLE S3. Number of Determinants in Hierarchy-, Excitation, and Seniority-Based CI Routes, as well as in Full CI, for HF, $H_8$, and ethylene, with the cc-pVDZ basis set and frozen-core approximation.

| method | HF | $H_8$ | ethylene |
|---|---:|---:|---:|
| RHF | 1 | 1 | 1 |
| CIS | 113 | 289 | 409 |
| CISD | 4 341 | 28 585 | 58 855 |
| CISDT | 68 405 | 1 174 345 | 3 731 535 |
| CISDTQ | 531 595 | 23 805 835 | 124 764 480 |
| CIs0 | 3 060 | 91 390 | 3 838 380 |
| CIs2 | 174 420 | 13 251 550 | 786 867 900 |
| CIs4 | 1 845 180 | 358 705 750 | 33 086 835 600 |
| hCI1 | 169 | 433 | 613 |
| hCI1.5 | 1 065 | 5 905 | 8 365 |
| hCI2 | 9 255 | 62 605 | 134 590 |
| hCI2.5 | 55 119 | 879 085 | 1 952 230 |
| hCI3 | 227 109 | 5 659 525 | 17 306 800 |
| hCI3.5 | 856 101 | 40 616 965 | 163 795 120 |
| hCI4 | 2 216 460 | 213 974 380 | 1 112 401 240 |
| FCI | 9 363 600 | 8 352 132 100 | 14 733 161 024 400 |

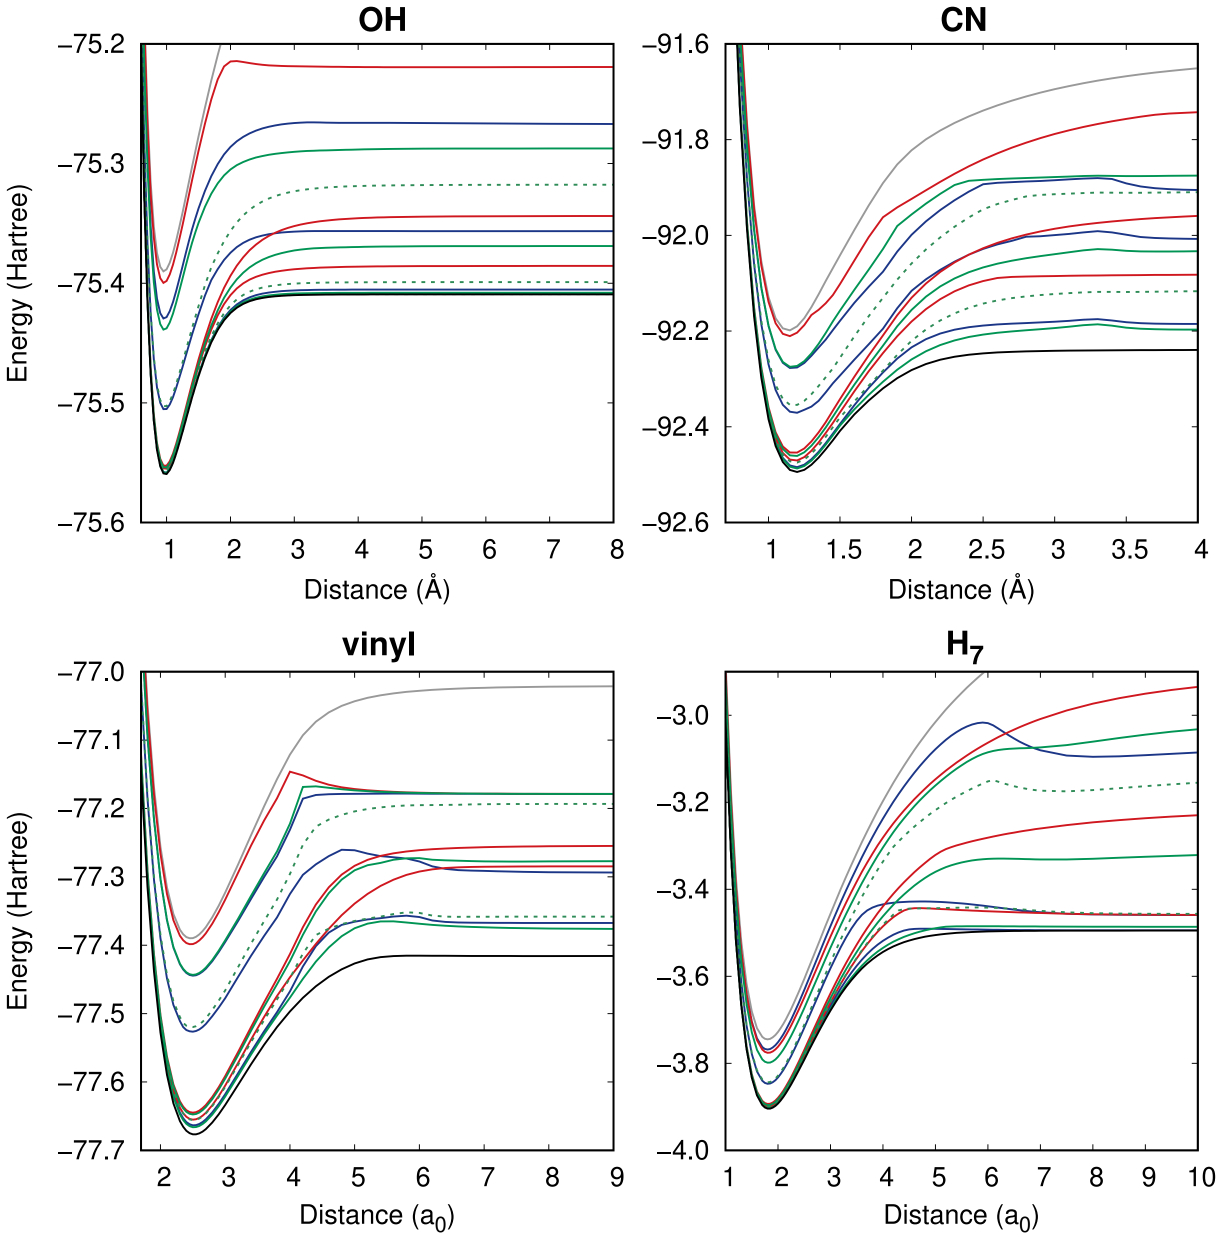


FIG. S1. Potential energy curves for OH, CN, vinyl, and $H_7$, according to restricted open-shell HF (gray), FCI (black), hCI (green) (dashed lines for half-integer $h$), eCI (red), and sCI (blue) models, with the cc-pVDZ basis set and frozen-core approximation.

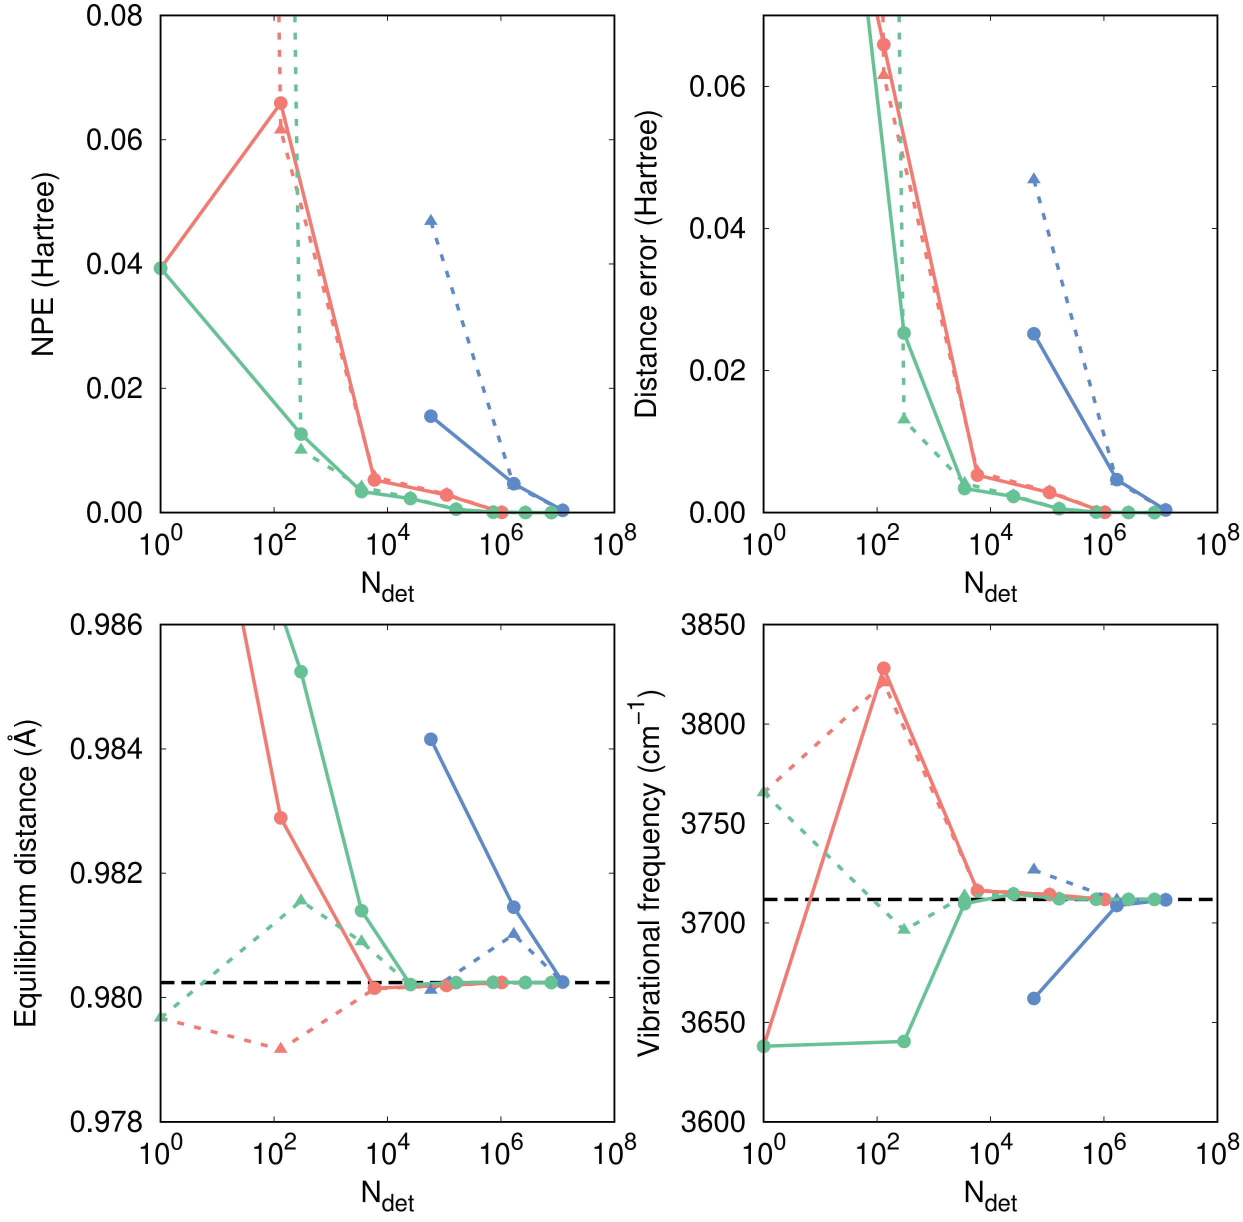


FIG. S2. Non-parallelity error (NPE), distance error, equilibrium distance, and vibrational frequency, for OH, as a function of the number of determinants ($N_{\text{det}}$), according to hCI (green), eCI (red) and sCI (blue) models, with the standard (full lines with circles) and renormalized (dashed lines with triangles) EN2 perturbative correction. The dashed lines represent the FCI results.

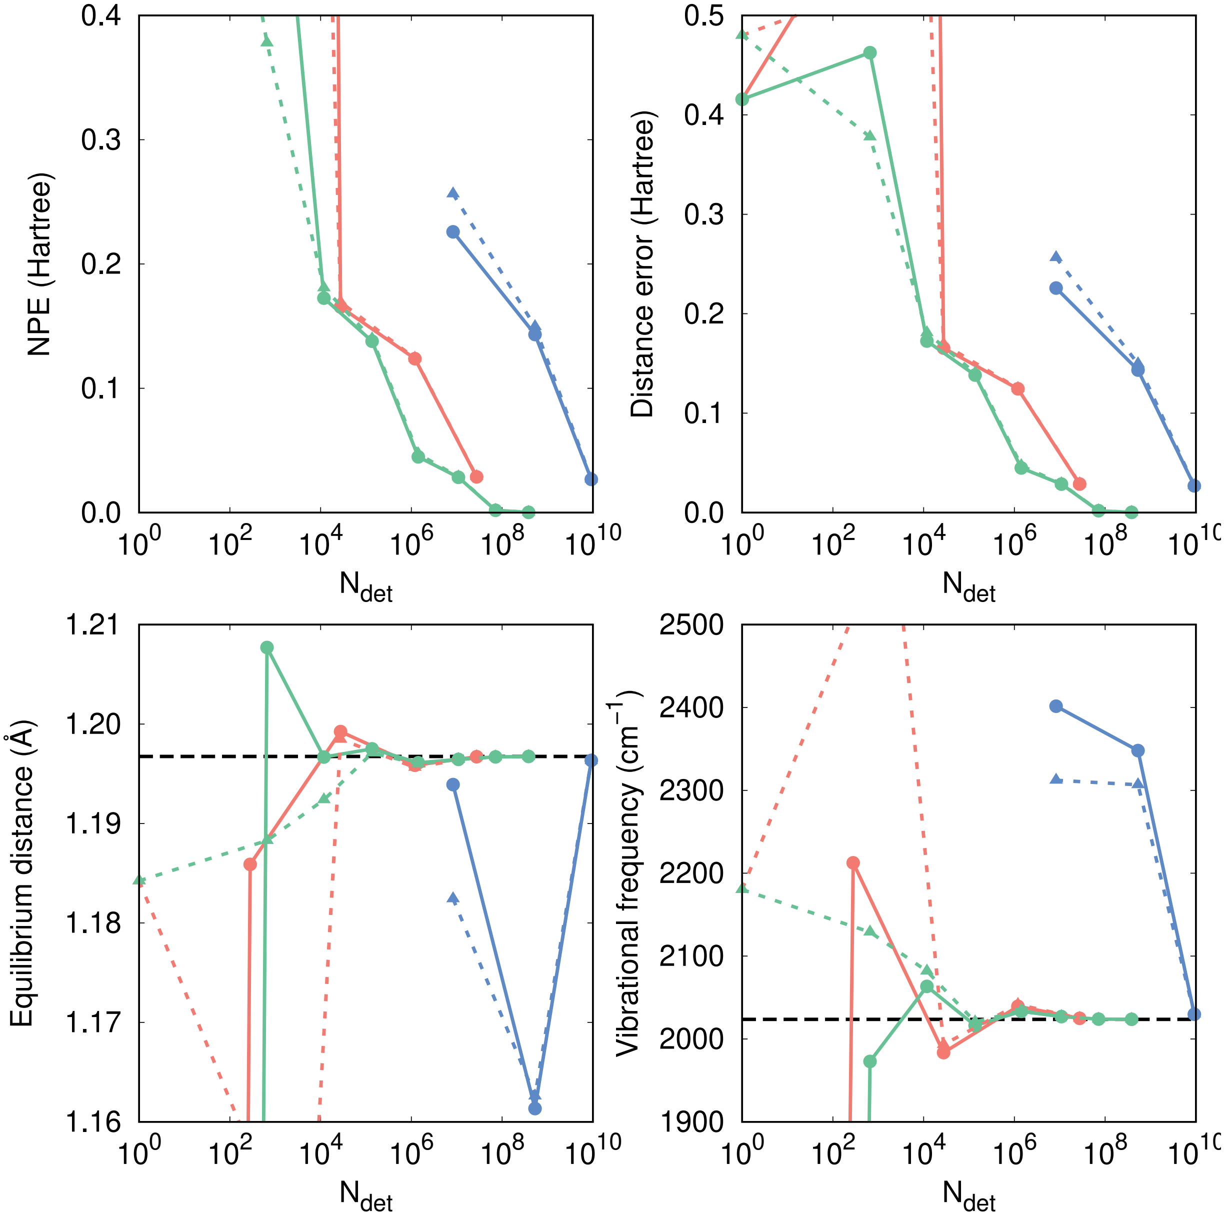


FIG. S3. Non-parallelity error (NPE), distance error, equilibrium distance, and vibrational frequency, for CN, as functions of the number of determinants ($N_{\text{det}}$), according to hCI (green), eCI (red) and sCI (blue) models, with the standard (full lines with circles) and renormalized (dashed lines with triangles) EN2 perturbative correction. The dashed lines represent the FCI results.

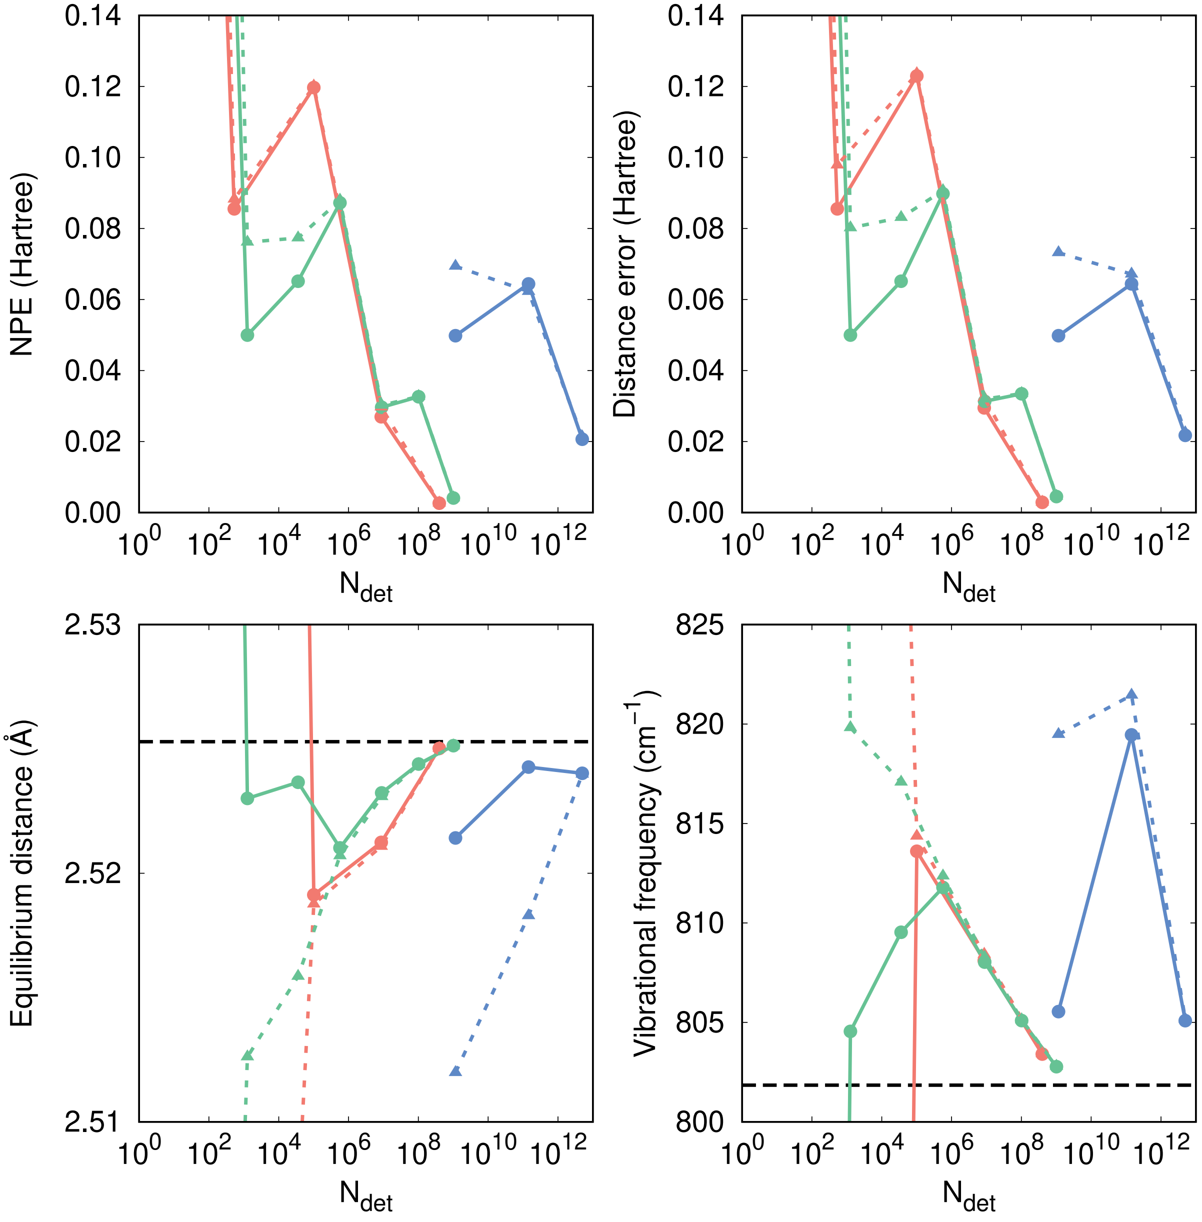


FIG. S4. Non-parallelity error (NPE), distance error, equilibrium distance, and vibrational frequency, for vinyl, as functions of the number of determinants ($N_{\text{det}}$), according to hCI (green), eCI (red) and sCI (blue) models, with the standard (full lines with circles) and renormalized (dashed lines with triangles) EN2 perturbative correction. The dashed lines represent the FCI results.

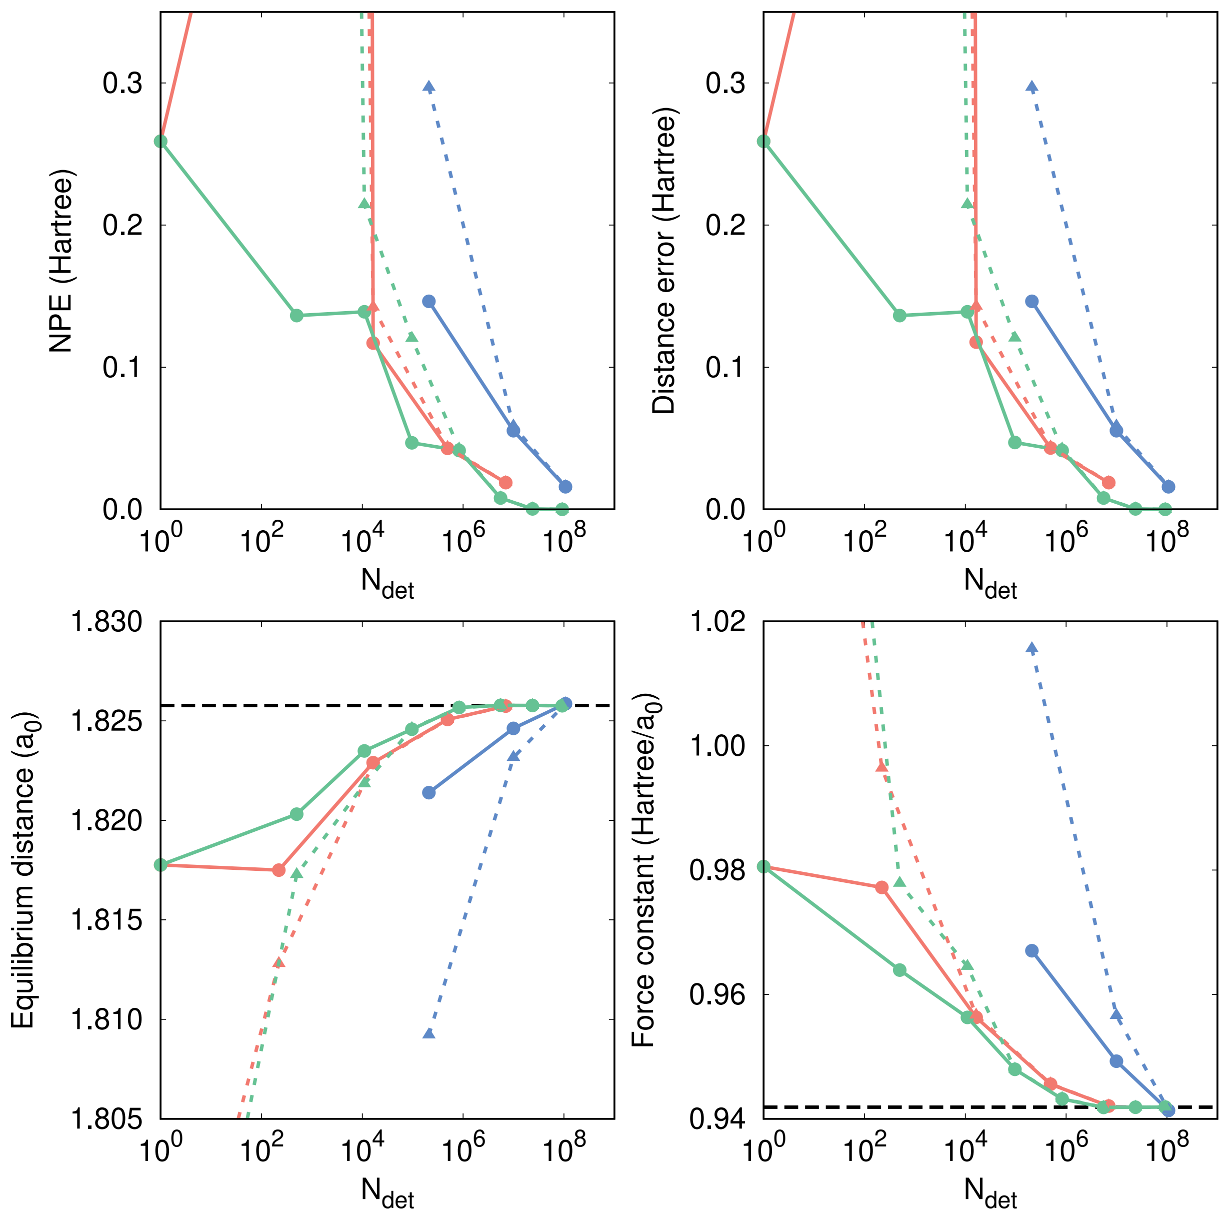


FIG. S5. Non-parallelity error (NPE), distance error, equilibrium distance, and force constant, for $H_7$, as functions of the number of determinants ($N_{\text{det}}$), according to hCI (green), eCI (red) and sCI (blue) models, with the standard (full lines with circles) and renormalized (dashed lines with triangles) EN2 perturbative correction. The dashed lines represent the FCI results.

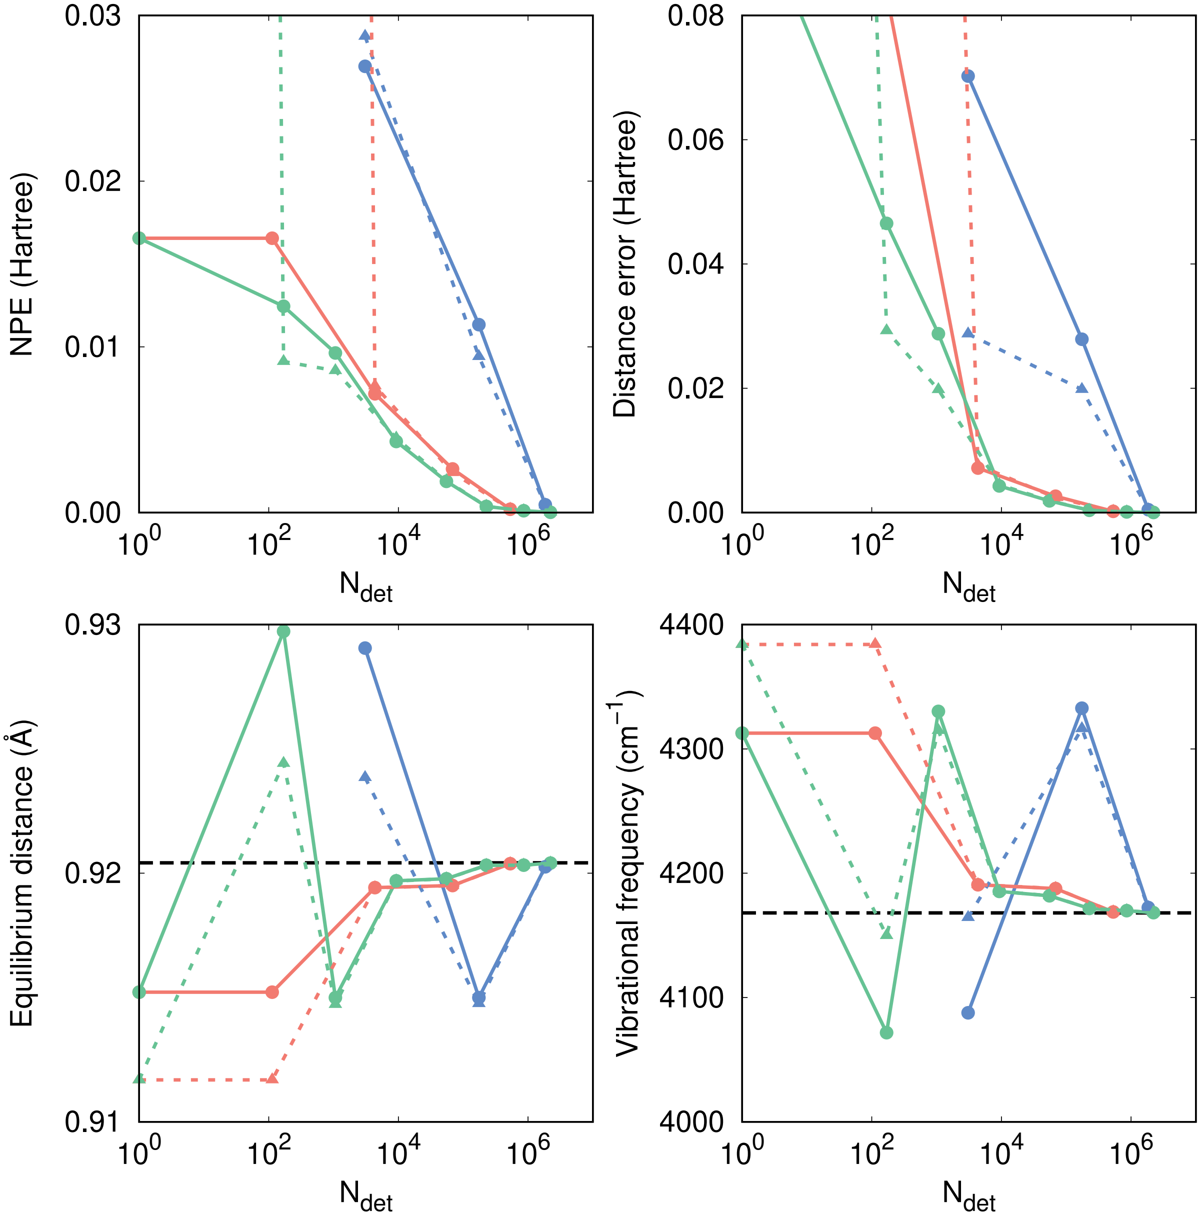


FIG. S6. Non-parallelity error (NPE), distance error, equilibrium distance, and vibrational frequency, for HF, as functions of the number of determinants ($N_{\text{det}}$), according to hCI (green), eCI (red) and sCI (blue) models, with the standard (full lines with circles) and renormalized (dashed lines with triangles) EN2 perturbative correction. The dashed lines represent the FCI results.

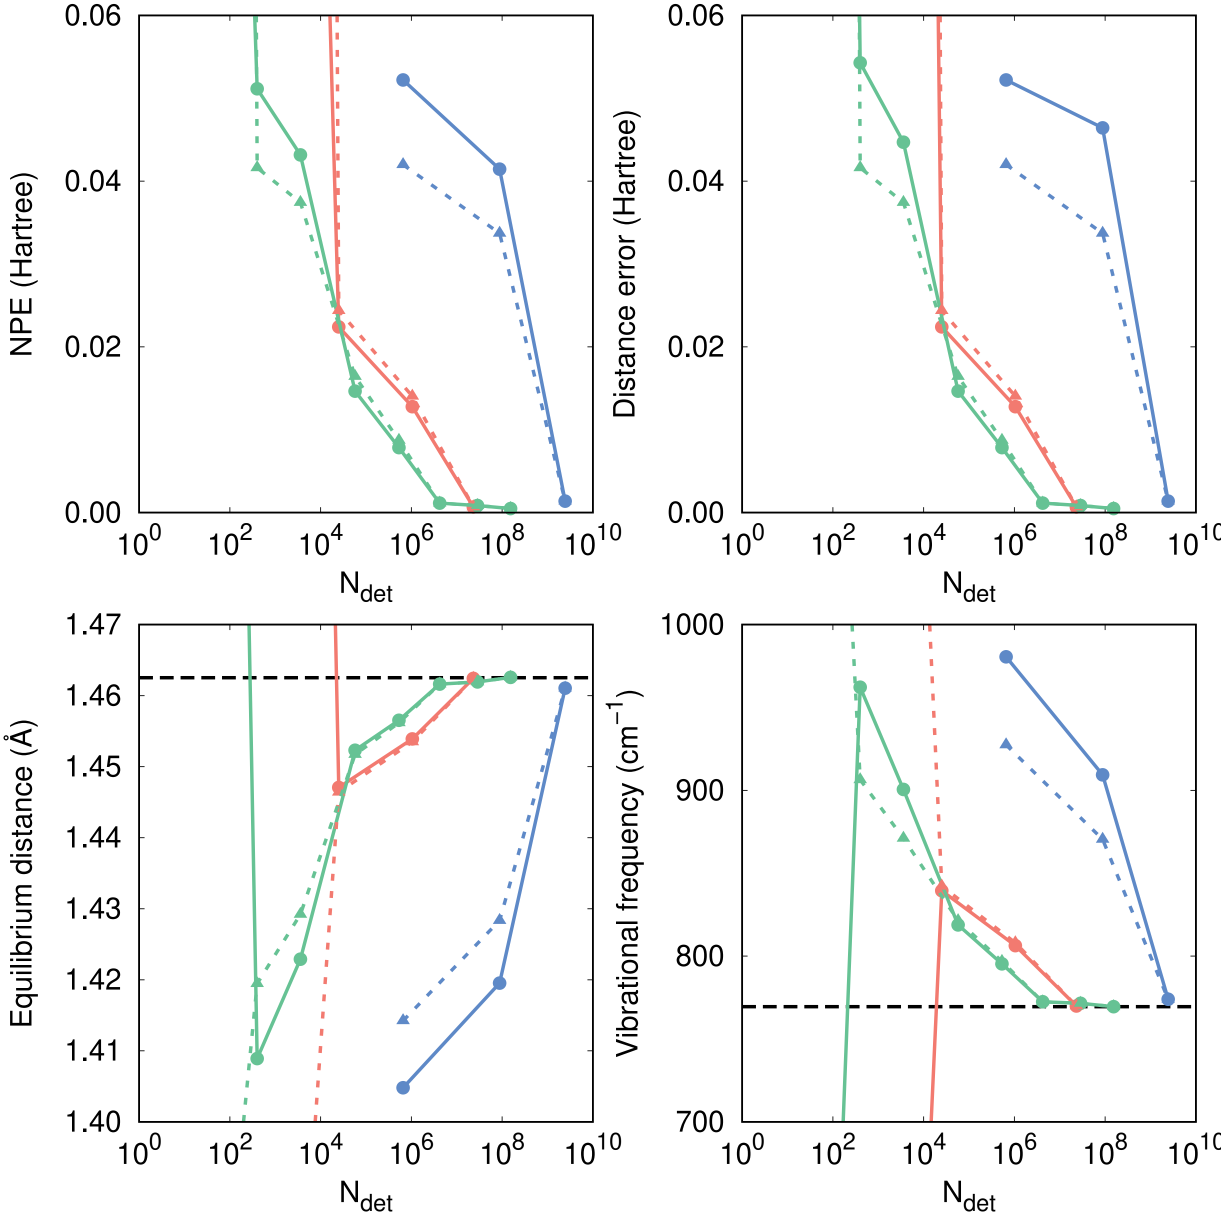


FIG. S7. Non-parallelity error (NPE), distance error, equilibrium distance, and vibrational frequency, for $F_2$, as functions of the number of determinants ($N_{\text{det}}$), according to hCI (green), eCI (red) and sCI (blue) models, with the standard (full lines with circles) and renormalized (dashed lines with triangles) EN2 perturbative correction. The dashed lines represent the FCI results.

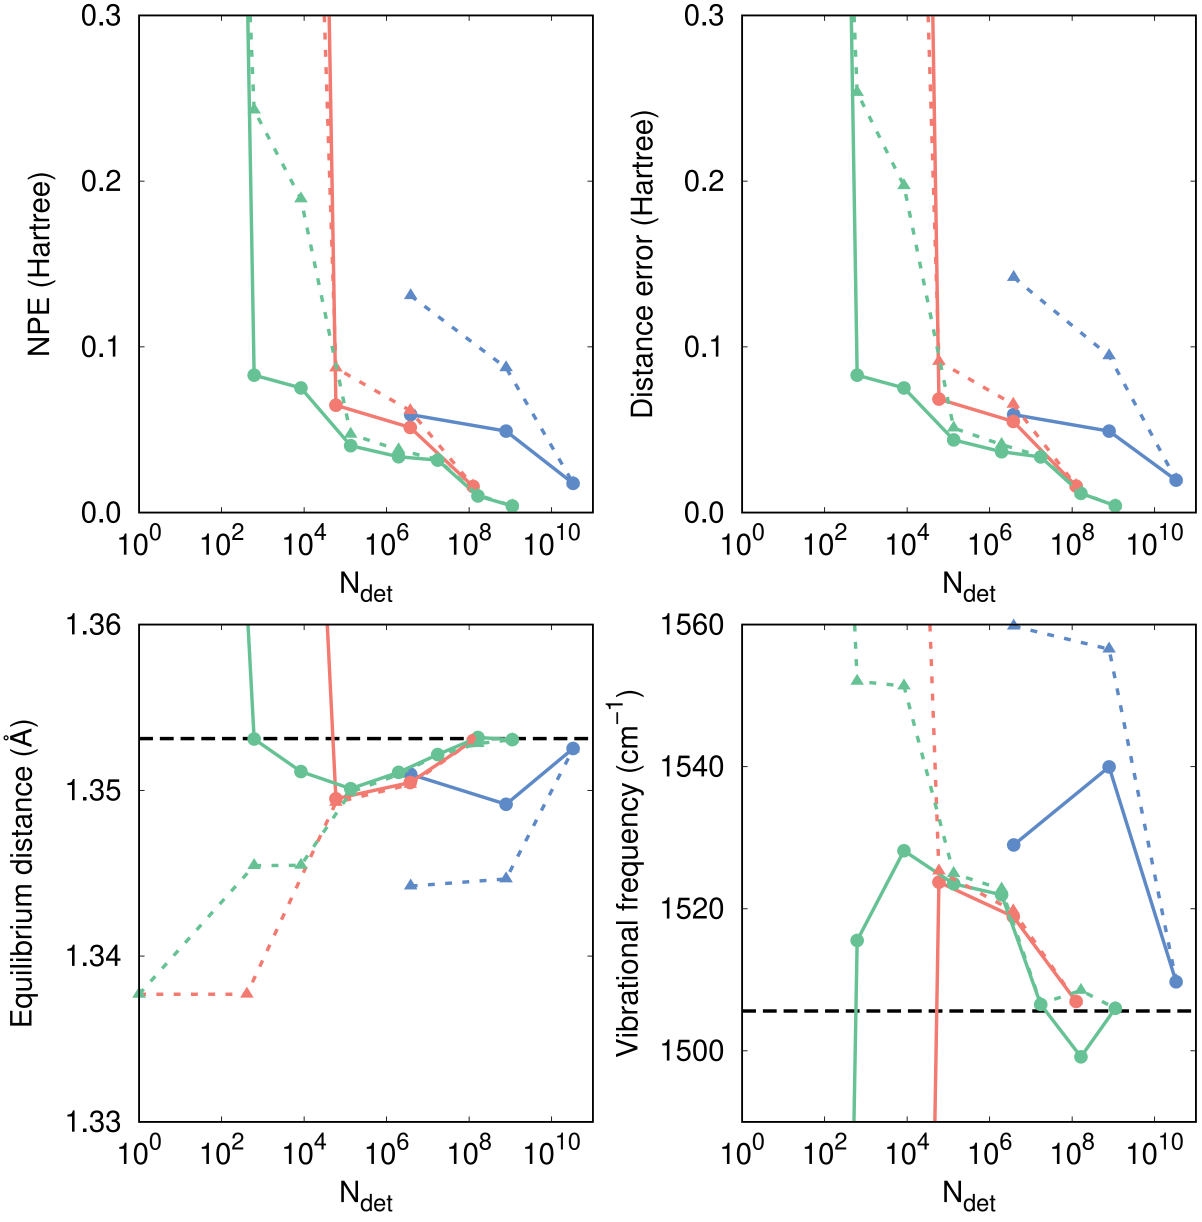


FIG. S8. Non-parallelity error (NPE), distance error, equilibrium distance, and vibrational frequency, for ethylene, as functions of the number of determinants ($N_{\text{det}}$), according to hCI (green), eCI (red) and sCI (blue) models, with the standard (full lines with circles) and renormalized (dashed lines with triangles) EN2 perturbative correction. The dashed lines represent the FCI results.

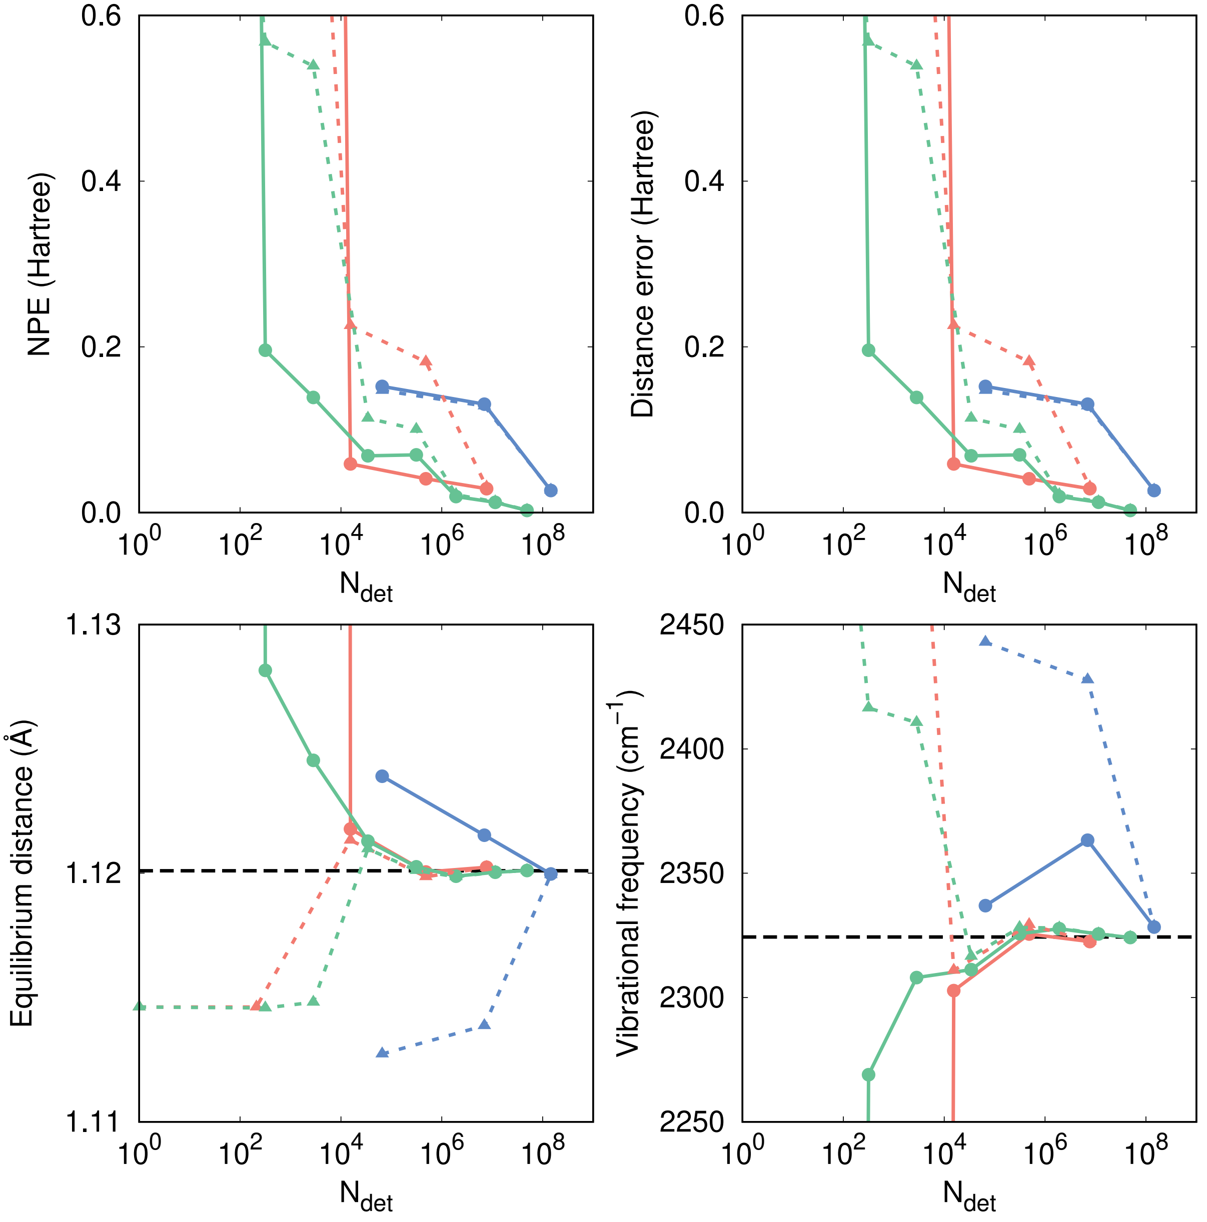


FIG. S9. Non-parallelity error (NPE), distance error, equilibrium distance, and vibrational frequency, for $N_2$, as functions of the number of determinants ($N_{\mathrm{det}}$), according to hCI (green), eCI (red) and sCI (blue) models, with the standard (full lines with circles) and renormalized (dashed lines with triangles) EN2 perturbative correction. The dashed lines represent the FCI results.

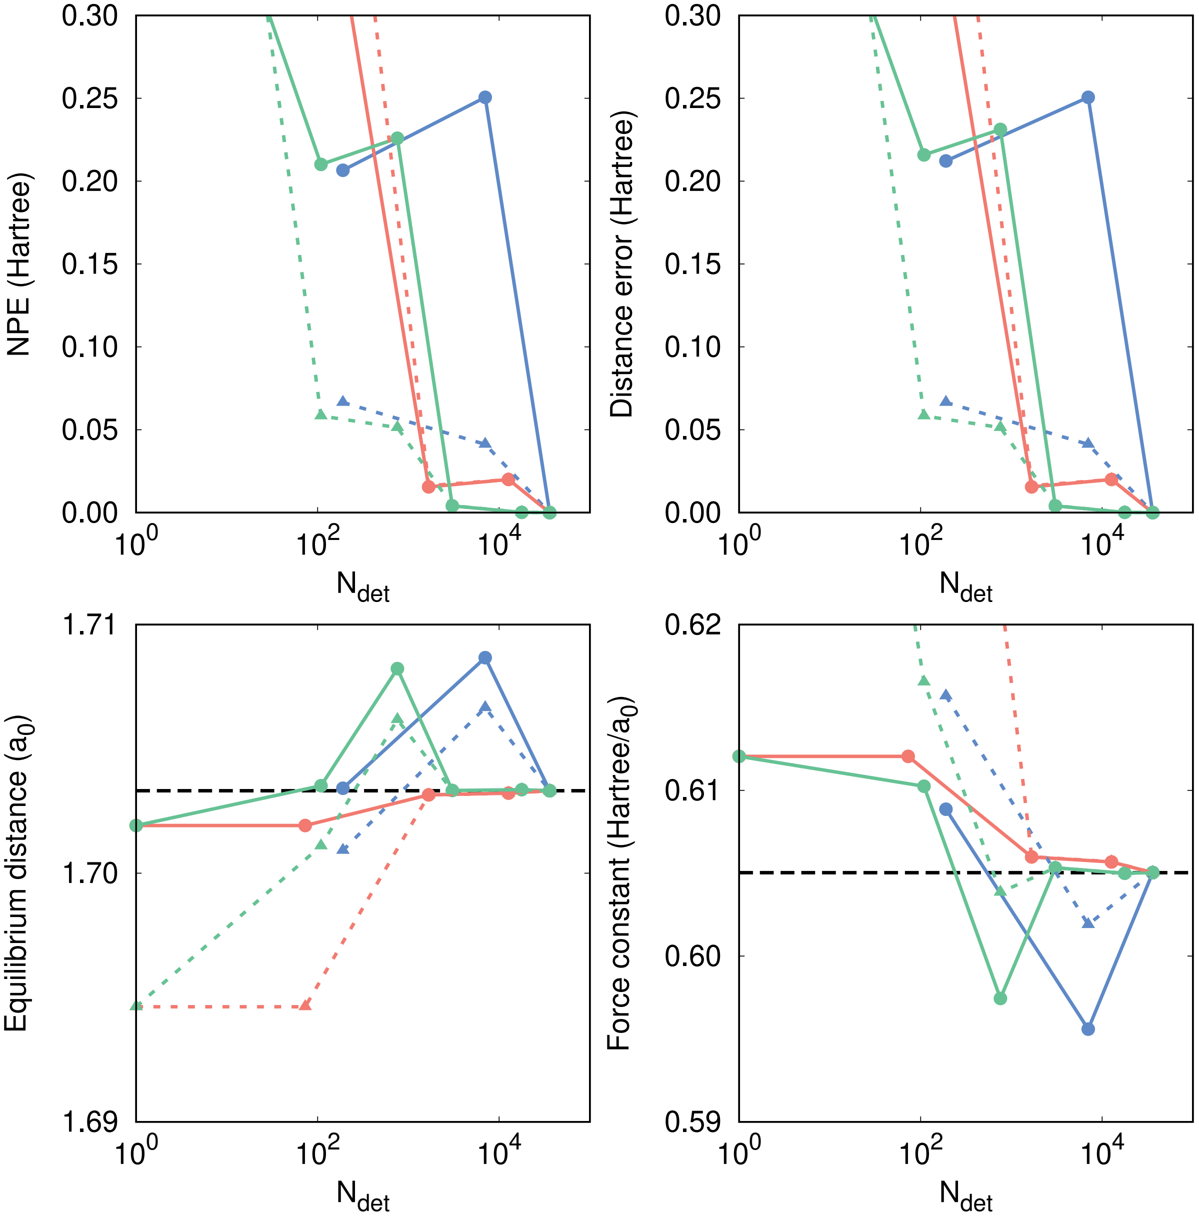


FIG. S10. Non-parallelity error (NPE), distance error, equilibrium distance, and force constant, for $H_4$, as functions of the number of determinants ($N_{\text{det}}$), according to hCI (green), eCI (red) and sCI (blue) models, with the standard (full lines with circles) and renormalized (dashed lines with triangles) EN2 perturbative correction. The dashed lines represent the FCI results.

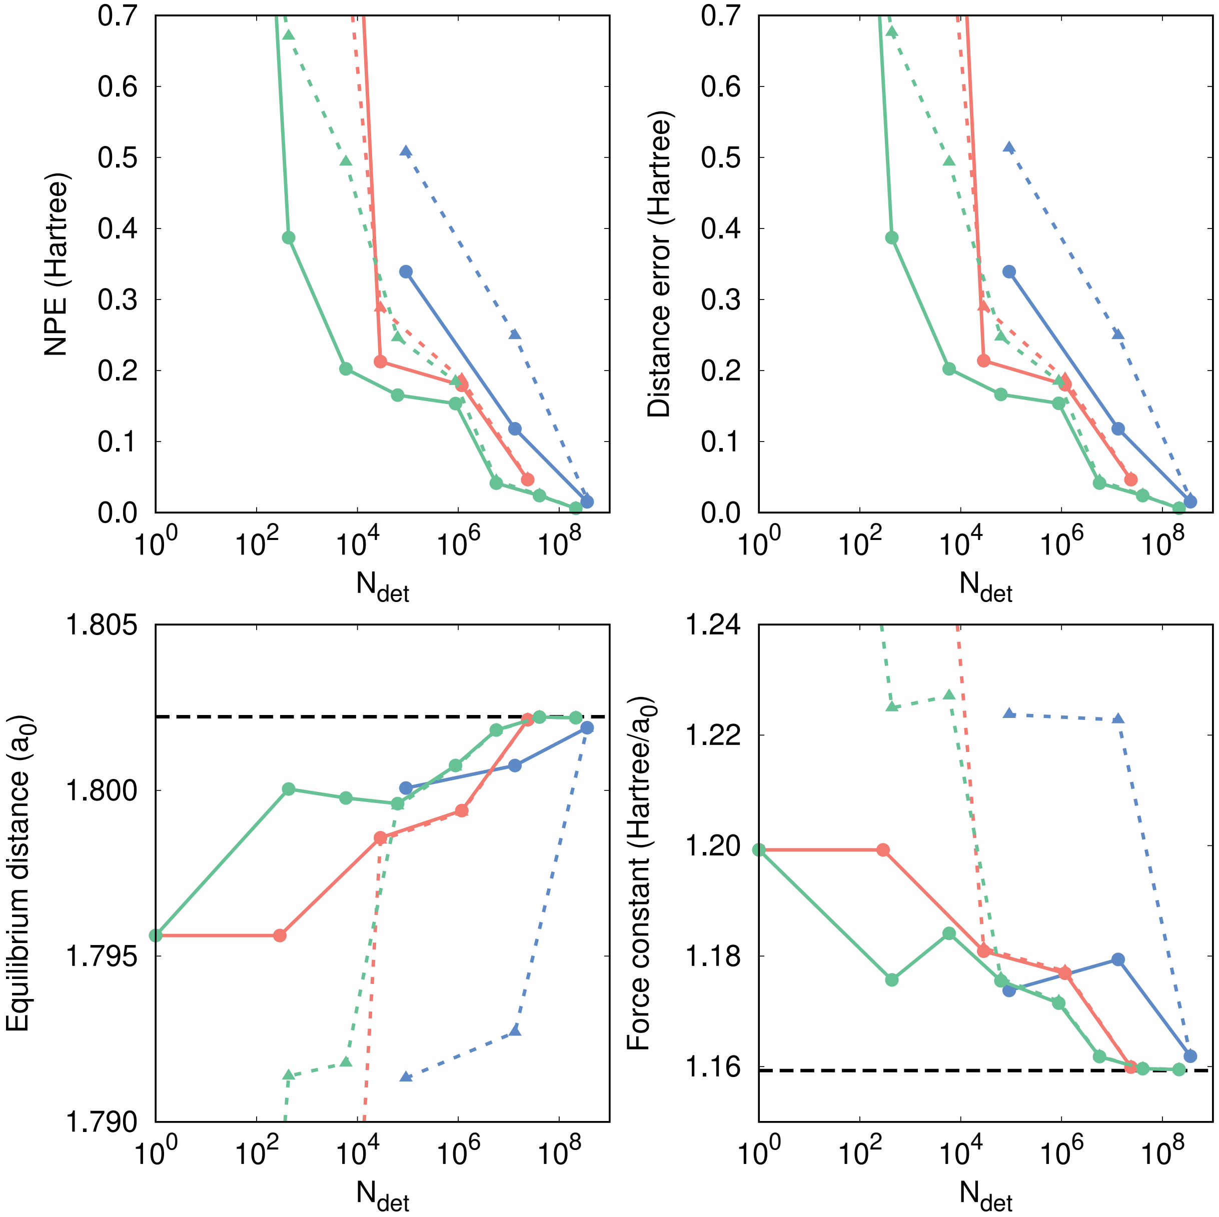


FIG. S11. Non-parallelity error (NPE), distance error, equilibrium distance, and force constant, for $H_8$, as functions of the number of determinants ($N_{\text{det}}$), according to hCI (green), eCI (red) and sCI (blue) models, with the standard (full lines with circles) and renormalized (dashed lines with triangles) EN2 perturbative correction. The dashed lines represent the FCI results.

## REFERENCES


[1] Loos, P. F.; Scemama, A.; Blondel, A.; Garniron, Y.; Caffarel, M.; Jacquemin, D. A Mountaineering Strategy to Excited States: Highly Accurate Reference Energies and Benchmarks. *J. Chem. Theory Comput.* **2018**, *14*, 4360.

[2] Loos, P.-F.; Scemama, A.; Boggio-Pasqua, M.; Jacquemin, D. Mountaineering Strategy to Excited States: Highly Accurate Energies and Benchmarks for Exotic Molecules and Radicals. *J. Chem. Theory Comput.* **2020**, *16*, 3720–3736.
